# Supplementary material for: Performance of the LHCb RICH detector at the LHC
Source: arXiv:1211.6759 source file (2013-09-17)
Supplement: Supplementary file 1 [file appendix.tex]

\vspace*{2cm}

{\noindent\bf\Large Appendix}

\appendix

\section{Appendix A}

Extra Blah...
